# Supplementary material for: The temporal overfitting problem with applications in wind power curve modeling
Source: arXiv:2012.01349 source file (2022-04-04)
Supplement: Supplementary file 1 [file SupplementaryMaterial.pdf]

# Supplementary Material for “The temporal overfitting problem with applications in wind power curve modeling”

Abhinav Prakash, Rui Tuo, and Yu Ding  
Department of Industrial and Systems Engineering  
Texas A&M University

## S1 Results with different covariance functions

Figure 1 presents the root mean square error (RMSE) using four different covariance functions—squared exponential, Matérn with  $\nu = 2.5$ , Matérn with  $\nu = 1.5$ , and exponential kernel. Matérn with  $\nu = 1.5$  in general performs the best.

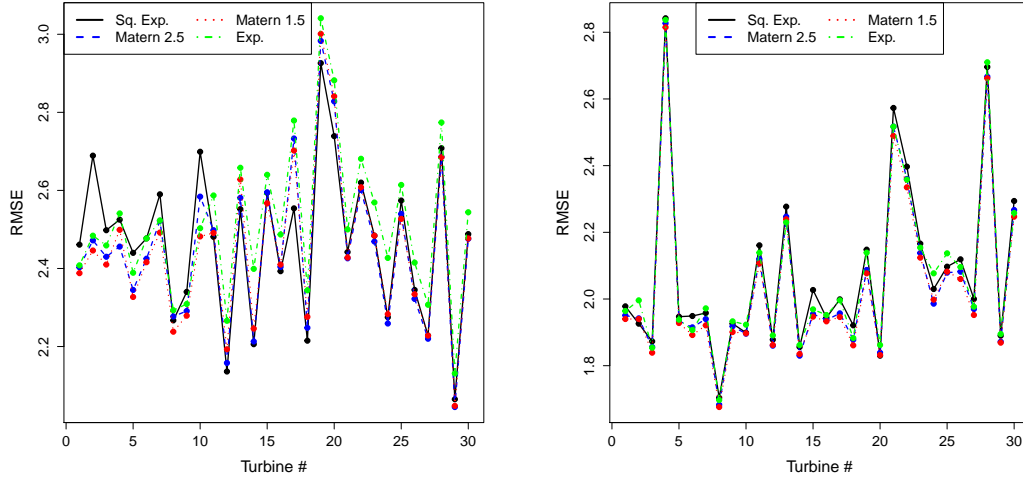

Figure 1: Root mean square error using different covariance function with tempGP method on test dataset  $\mathcal{T}_2$  (left panel) and  $\mathcal{T}_3$  (right panel).

## S2 PACF plots for WT1

Figure 2 presents the partial autocorrelation function (PACF) plot for all the input variables and the response for WT1, clearly indicating significant temporal autocorrelation upto several lags for each of the variables.

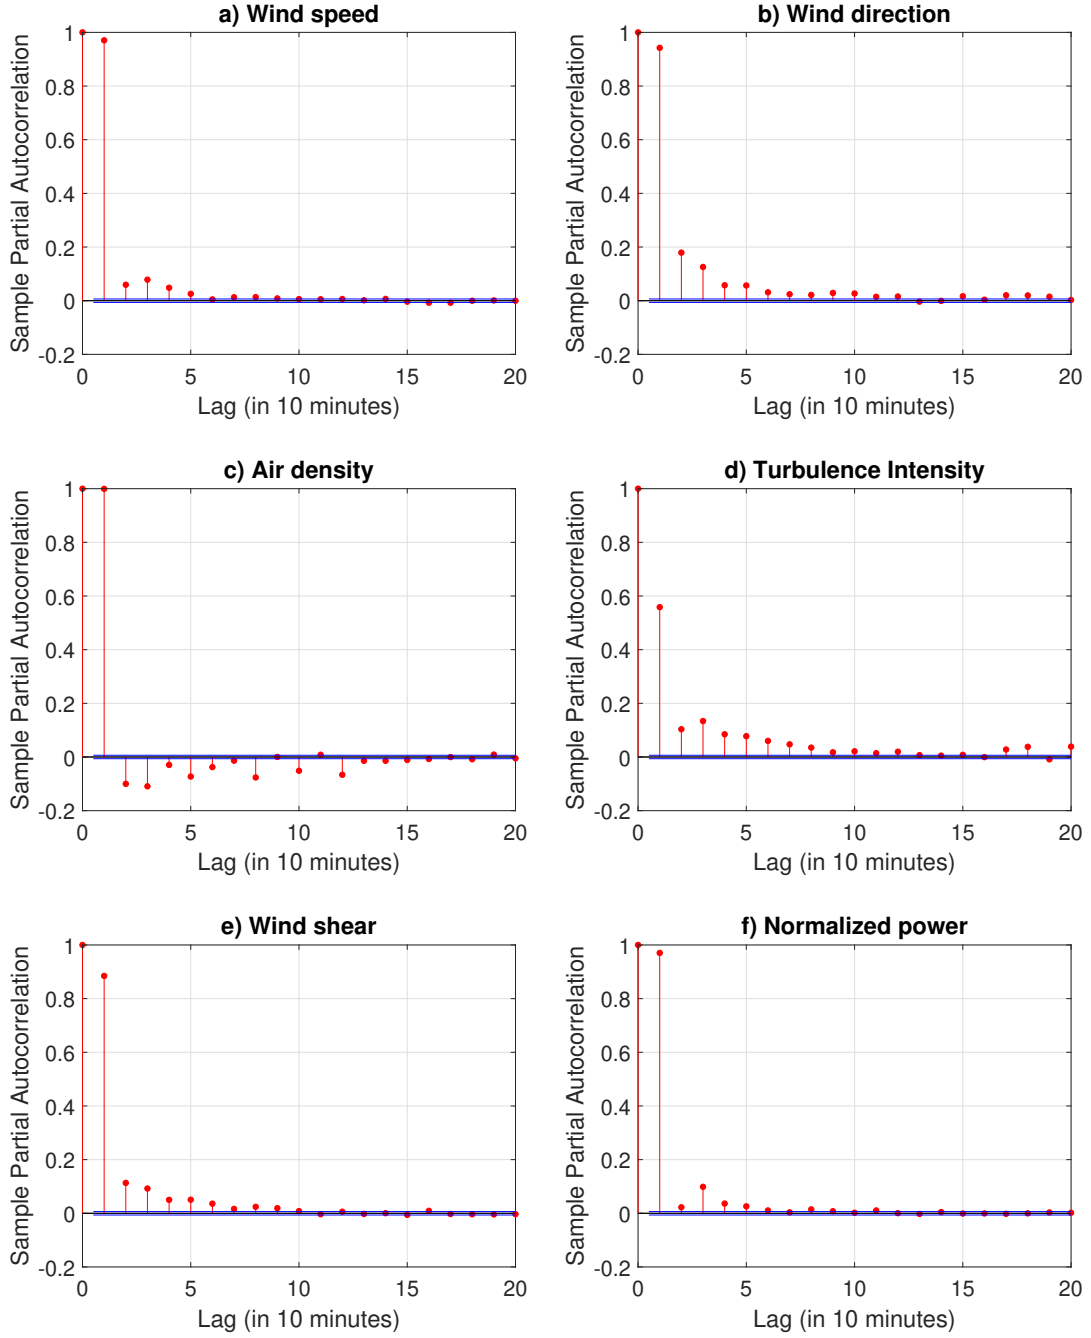

Figure 2: Sample partial autocorrelation function plots for WT1: a) wind speed, b) wind direction, c) air density, d) turbulence intensity, e) wind shear and f) normalized power.

### S3 Hyperparameter estimates

Table 1 presents the hyperparameter estimates for the tempGP method.

Table 1: Hyperparameter estimates for the tempGP method.

| Turbine | $\beta$ | $\sigma_f$ | $\sigma_u$ | $\theta_V$ | $\theta_\rho$ | $\theta_I$ | $\theta_S$ | $\theta_{\sin_D}$ | $\theta_{\cos_D}$ |
|---------|---------|------------|------------|------------|---------------|------------|------------|-------------------|-------------------|
| 1       | 34.09   | 36.74      | 1.95       | 4.78       | 45.83         | 15.24      | 54.43      | 544.99            | 158.95            |
| 2       | 32.93   | 36.22      | 2.13       | 4.53       | 31.02         | 12.01      | 94.58      | 218.99            | 208.32            |
| 3       | 33.11   | 37.99      | 1.94       | 4.42       | 46.17         | 11.99      | 85.81      | 69393.62          | 307.21            |
| 4       | 30.8    | 40.66      | 1.97       | 5.18       | 41.48         | 15.15      | 78.2       | 1337.42           | 216.4             |
| 5       | 32.22   | 39.03      | 1.86       | 4.66       | 46.2          | 11.3       | 132.76     | 1322.21           | 1394.42           |
| 6       | 30.6    | 39.73      | 2.02       | 4.87       | 45.07         | 13.46      | 67.69      | 45027.03          | 207.89            |
| 7       | 29.17   | 39.39      | 2.21       | 4.61       | 40.37         | 12.41      | 78         | 132237.32         | 582.09            |
| 8       | 29.68   | 37.38      | 1.75       | 5.14       | 36.97         | 12.24      | 76.78      | 70929.75          | 146.45            |
| 9       | 29.25   | 39.01      | 2.08       | 5.03       | 65.07         | 13.73      | 64.42      | 472.78            | 164.14            |
| 10      | 29.63   | 41.24      | 2.11       | 5.24       | 53.09         | 9.09       | 136.55     | 260.54            | 196.95            |
| 11      | 33.1    | 35.56      | 2.04       | 4.28       | 21.75         | 17.11      | 39.44      | 248872.8          | 68.72             |
| 12      | 30.88   | 35.93      | 1.85       | 4.55       | 32.12         | 14.18      | 205.42     | 1752.95           | 81.4              |
| 13      | 31.7    | 36.73      | 2.04       | 4.8        | 21.82         | 15.94      | 46.71      | 65464.45          | 37.02             |
| 14      | 29.66   | 36.16      | 1.98       | 4.45       | 27.96         | 14.02      | 40.91      | 6227.06           | 94.95             |
| 15      | 31.38   | 36.06      | 2.26       | 4.11       | 24.3          | 14.77      | 31.8       | 187497            | 117.83            |
| 16      | 33.84   | 35.85      | 2.05       | 4.52       | 19.41         | 14.84      | 49.69      | 814.28            | 34.37             |
| 17      | 35.13   | 36.27      | 2.56       | 4.44       | 16.92         | 17.43      | 44.11      | 210.91            | 26.19             |
| 18      | 31.99   | 38.4       | 2.07       | 4.36       | 30.09         | 18.96      | 49.21      | 1544.16           | 200.82            |
| 19      | 33.76   | 35.55      | 2.63       | 4.06       | 18.28         | 16.11      | 36.84      | 392903.68         | 59.64             |
| 20      | 31.92   | 35.95      | 2.19       | 4.26       | 21.81         | 11.04      | 74.69      | 573.31            | 84.37             |
| 21      | 31.82   | 34.4       | 2.25       | 4.15       | 27.15         | 12.64      | 51.71      | 406.72            | 216.1             |
| 22      | 35.1    | 37.75      | 2.49       | 4.18       | 24.21         | 16.13      | 53.12      | 293.18            | 1274.85           |
| 23      | 33.54   | 39.8       | 2.62       | 4.37       | 27.44         | 15.28      | 59.05      | 205.69            | 438.89            |
| 24      | 42.27   | 41.04      | 2.27       | 3.95       | 19.26         | 26.24      | 61.37      | 811.3             | 387.51            |
| 25      | 32.44   | 39.45      | 2.45       | 4.47       | 23.19         | 13.79      | 79.49      | 538.7             | 378.64            |
| 26      | 31.92   | 36.01      | 2.33       | 4.48       | 23.54         | 15.08      | 58.98      | 37.5              | 208.53            |
| 27      | 35.27   | 38.14      | 2.32       | 4.3        | 25.07         | 16.42      | 58.35      | 470.12            | 199.82            |
| 28      | 37.86   | 39.96      | 2.55       | 4.37       | 24.79         | 17.02      | 62.16      | 174969.55         | 159906.92         |
| 29      | 35.64   | 37.8       | 2.09       | 4.35       | 25.59         | 15.39      | 68.24      | 459.73            | 293.57            |
| 30      | 38.88   | 39.95      | 2.36       | 4.44       | 25.78         | 22.25      | 60.06      | 253.03            | 717.34            |

## S4 RMSE for Case Study II

Tables 2 and 3 presents the root mean square error (RMSE) for all the thirty turbine in Case Study II.

Table 2: Actual RMSE for different methods on test data  $\mathcal{T}_2$

| Turbine | Binning | kNN  | AMK  | regGP | tempGP | CVc-kNN | TS-kNN | PW-AMK |
|---------|---------|------|------|-------|--------|---------|--------|--------|
| 1       | 3.65    | 5.73 | 4.16 | 6.04  | 2.39   | 4.68    | 5.04   | 4.08   |
| 2       | 4.19    | 5.72 | 3.86 | 6.46  | 2.45   | 4.98    | 5.07   | 3.81   |
| 3       | 3.58    | 5.62 | 3.67 | 6.48  | 2.41   | 4.39    | 4.77   | 3.71   |
| 4       | 3.54    | 5.61 | 3.64 | 6.3   | 2.5    | 4.37    | 4.56   | 3.55   |
| 5       | 3.66    | 6.04 | 4.93 | 7.57  | 2.33   | 4.99    | 5.47   | 4.85   |
| 6       | 3.88    | 5.33 | 4.67 | 7.22  | 2.42   | 4.26    | 4.57   | 4.55   |
| 7       | 3.72    | 5.41 | 3.61 | 6.33  | 2.49   | 3.16    | 3.16   | 3.56   |
| 8       | 3.27    | 5.9  | 3.4  | 5.71  | 2.24   | 4.23    | 4.49   | 3.34   |
| 9       | 2.95    | 5.21 | 2.87 | 6.15  | 2.28   | 2.75    | 2.75   | 2.87   |
| 10      | 3.73    | 5.89 | 4.46 | 7.12  | 2.48   | 4.82    | 4.79   | 4.43   |
| 11      | 3.5     | 4.26 | 5.58 | 5.7   | 2.49   | 3.85    | 3.88   | 5.53   |
| 12      | 2.56    | 3.73 | 4.73 | 5.27  | 2.19   | 3.6     | 2.39   | 4.68   |
| 13      | 2.85    | 4.02 | 5.46 | 5.54  | 2.63   | 3.81    | 2.66   | 5.38   |
| 14      | 3.2     | 3.94 | 5.7  | 5.34  | 2.25   | 3.6     | 3.54   | 5.67   |
| 15      | 3.89    | 4.03 | 5.49 | 5.47  | 2.57   | 3.81    | 3.61   | 5.48   |
| 16      | 3.13    | 3.91 | 5.19 | 5     | 2.41   | 3.66    | 3.5    | 5.15   |
| 17      | 3.22    | 4.06 | 5.63 | 6.08  | 2.7    | 3.66    | 3.55   | 5.54   |
| 18      | 2.93    | 4.59 | 5.25 | 5.1   | 2.28   | 3.86    | 3.69   | 5.22   |
| 19      | 3.99    | 5.58 | 5.48 | 6.27  | 3      | 3.87    | 3.94   | 5.43   |
| 20      | 3.48    | 4.31 | 4.88 | 4.96  | 2.84   | 4.25    | 4.1    | 4.85   |
| 21      | 2.7     | 2.9  | 3.33 | 3.4   | 2.43   | 2.83    | 2.86   | 3.29   |
| 22      | 3.24    | 4.69 | 3.46 | 3.82  | 2.61   | 2.96    | 3.04   | 3.43   |
| 23      | 2.95    | 4.49 | 3.51 | 3.93  | 2.48   | 2.79    | 2.82   | 3.46   |
| 24      | 2.86    | 3.5  | 4.34 | 3.88  | 2.28   | 2.81    | 2.78   | 4.69   |
| 25      | 3.24    | 2.9  | 3.52 | 3.6   | 2.53   | 3.02    | 3.01   | 3.5    |
| 26      | 2.81    | 2.74 | 2.87 | 3.1   | 2.33   | 2.6     | 2.6    | 2.85   |
| 27      | 2.89    | 2.71 | 3.13 | 3.16  | 2.23   | 2.69    | 2.71   | 3.09   |
| 28      | 3.41    | 3.14 | 3.44 | 3.6   | 2.68   | 3.07    | 3.11   | 3.39   |
| 29      | 2.64    | 2.38 | 2.6  | 2.68  | 2.05   | 2.42    | 2.4    | 2.59   |
| 30      | 2.96    | 2.91 | 3.33 | 3.34  | 2.48   | 2.84    | 2.86   | 3.28   |

Table 3: Actual RMSE for different methods on test data  $\mathcal{T}_3$ 

| Turbine | Binning | kNN  | AMK  | regGP | tempGP | CVc-kNN | TS-kNN | PW-AMK |
|---------|---------|------|------|-------|--------|---------|--------|--------|
| 1       | 2.8     | 2.13 | 2.19 | 2.12  | 1.94   | 2.2     | 2.24   | 2.17   |
| 2       | 2.93    | 2.17 | 2.27 | 2.28  | 1.94   | 2.14    | 2.17   | 2.22   |
| 3       | 2.52    | 2.06 | 2.12 | 2.01  | 1.84   | 2.1     | 2.21   | 2.11   |
| 4       | 3.14    | 3.01 | 3.11 | 2.98  | 2.82   | 3.08    | 3.16   | 3.1    |
| 5       | 2.75    | 2.11 | 2.25 | 2.08  | 1.93   | 2.13    | 2.14   | 2.22   |
| 6       | 2.8     | 2.16 | 2.28 | 2.05  | 1.89   | 2.2     | 2.3    | 2.25   |
| 7       | 2.78    | 2.17 | 2.24 | 2.25  | 1.92   | 2.42    | 2.43   | 2.22   |
| 8       | 2.28    | 1.87 | 1.93 | 1.79  | 1.68   | 1.89    | 2.01   | 1.92   |
| 9       | 2.29    | 2.14 | 2.1  | 2.16  | 1.9    | 2.19    | 2.2    | 2.08   |
| 10      | 2.6     | 2.19 | 2.23 | 2.14  | 1.9    | 2.2     | 2.33   | 2.2    |
| 11      | 2.92    | 2.17 | 2.46 | 2.35  | 2.11   | 2.21    | 2.21   | 2.44   |
| 12      | 2.6     | 2.01 | 2.15 | 2.09  | 1.86   | 2.05    | 2.51   | 2.13   |
| 13      | 3.31    | 2.42 | 2.56 | 2.37  | 2.24   | 2.41    | 3.08   | 2.54   |
| 14      | 3.1     | 2.04 | 2.26 | 2.09  | 1.83   | 2.09    | 2.12   | 2.22   |
| 15      | 3.58    | 2.28 | 2.44 | 2.27  | 1.95   | 2.29    | 2.29   | 2.42   |
| 16      | 3.07    | 2.15 | 2.31 | 2.13  | 1.93   | 2.17    | 2.19   | 2.29   |
| 17      | 3.28    | 2.61 | 2.41 | 2.35  | 1.95   | 2.33    | 2.32   | 2.39   |
| 18      | 3.31    | 2.08 | 2.19 | 2.06  | 1.86   | 2.11    | 2.15   | 2.18   |
| 19      | 3.23    | 2.89 | 2.63 | 2.53  | 2.08   | 2.48    | 2.47   | 2.6    |
| 20      | 2.73    | 2.03 | 2.19 | 2.13  | 1.83   | 2.15    | 2.16   | 2.17   |
| 21      | 4.11    | 2.9  | 3.01 | 2.73  | 2.49   | 2.93    | 2.95   | 3.01   |
| 22      | 4.22    | 3.44 | 2.85 | 2.69  | 2.34   | 2.78    | 2.79   | 2.84   |
| 23      | 3.77    | 3.48 | 2.77 | 2.63  | 2.12   | 2.62    | 2.65   | 2.72   |
| 24      | 4.21    | 2.72 | 3.13 | 2.44  | 2      | 2.4     | 2.49   | 3.36   |
| 25      | 3.24    | 2.28 | 2.57 | 2.52  | 2.08   | 2.44    | 2.44   | 2.56   |
| 26      | 3.63    | 2.54 | 2.46 | 2.43  | 2.06   | 2.48    | 2.52   | 2.46   |
| 27      | 3.59    | 2.34 | 2.53 | 2.21  | 1.95   | 2.44    | 2.47   | 2.5    |
| 28      | 4.41    | 3    | 3.15 | 2.94  | 2.66   | 3.08    | 3.11   | 3.11   |
| 29      | 3.54    | 2.31 | 2.32 | 2.1   | 1.87   | 2.33    | 2.36   | 2.32   |
| 30      | 3.9     | 2.64 | 2.81 | 2.53  | 2.25   | 2.67    | 2.69   | 2.78   |

## S5 Prediction intervals

In order to gauge the uncertainty in the predictions, we plot the prediction intervals for our proposed method along with the actual observations. In order to make the plots legible, we sample 100 test points at random from the test set  $\mathcal{T}_2$ . The test points are vectors with six components (two for wind direction), but for plotting purpose, we use only wind speed input as the ‘x’-axis.

Figures 3 shows the 95% prediction interval for  $y$  along with the actual observations for Turbine 1, 11, 21, and 30 from Case Study II. Clearly, the proposed method provides reasonable inference in terms of uncertainty quantification. Other turbine datasets show similar pattern.

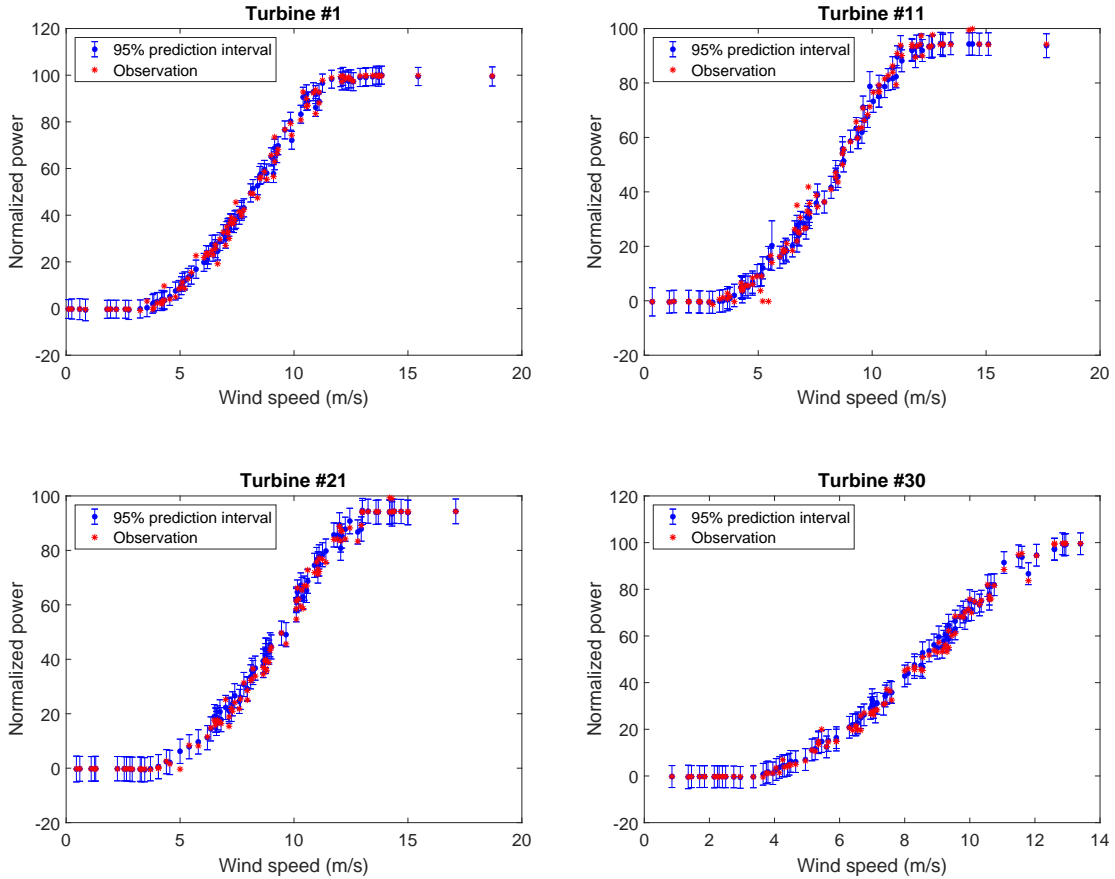

Figure 3: Prediction intervals for some of the test observations for: Turbine 1 (top left), Turbine 11 (top right), Turbine 21 (bottom left), Turbine 30 (bottom right).

## S6 Experiments on a simulated function

In order to validate our model’s efficacy, we apply our model to a simulated function. We consider a univariate function,  $f(x) = x^2$ . We start by sampling input points such that they are serially autocorrelated. To this end, we sequentially sample 100 linearly spaced points from the support  $[0, 10]$  and add noise to the samples. The PACF plot for  $x$  for one of the simulations is presented in Figure 4. Clearly, the PACF shows a similar pattern as shown in the inputs of the real wind turbine datasets (see Figure 2).

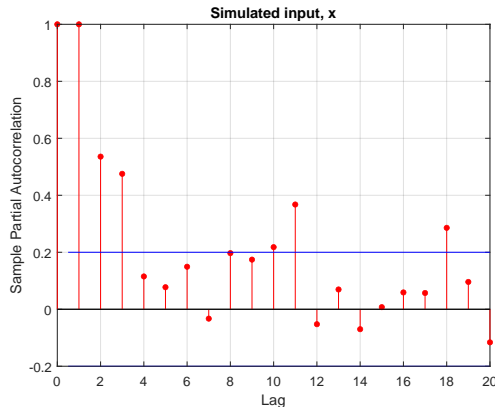

Figure 4: PACF plot for the simulated input,  $x$ , for one of the simulation runs.

Next, we sample serially autocorrelated errors from a zero mean Gaussian process (GP) with a Matérn covariance function with variance parameter  $\sigma_g = 10$  and smoothness parameter  $\nu = 1.5$ . We vary the lengthscale parameter  $\phi$  from 0.5 to 5 with an increment of 0.5 to get different strengths of autocorrelation in the errors. For each value of  $\phi$ , we simulate 100 training datasets with different random samples of input  $x$ , the autocorrelated error part  $g(t)$ , and the i.i.d. error part  $\epsilon$ . We plot the dataset, that is,  $(x, y)$  pair for one of the simulation runs in Figure 5. We fit a function on the simulated dataset using our proposed method (tempGP) and a regular version of GP (regGP) as described in the paper. Figure 6 shows the fit of tempGP and regGP on Figure 5’s dataset. The tempGP method provides a fit that is much closer to the true function as compared to regGP.

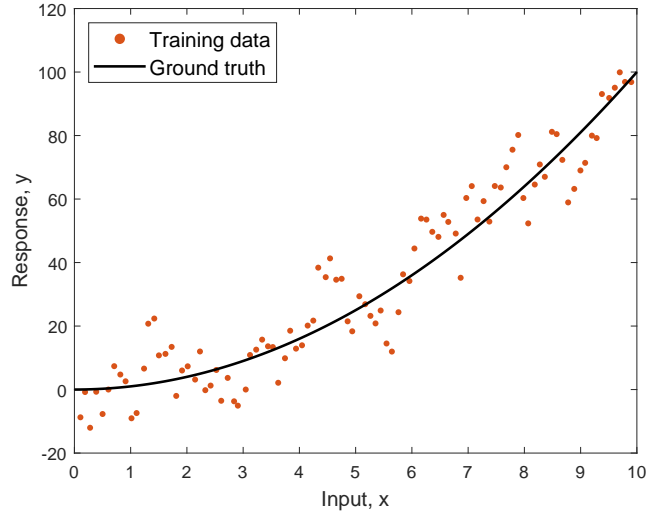

Figure 5: Simulated dataset for one of the simulation runs with lengthscale parameter  $\phi = 2.5$ .

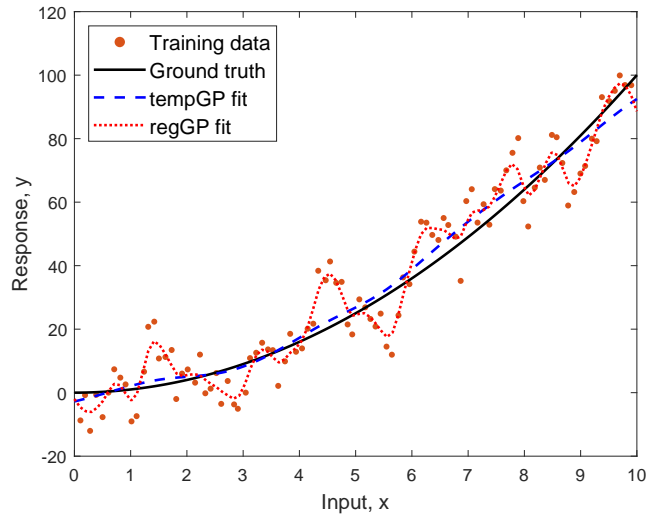

Figure 6: Fit of tempGP and regGP on the simulated dataset shown in Figure 5.

For each of the runs, we also simulate another set of dataset with different inputs and errors, to serve as testset. Using this testset, we then compare the root mean square error

Table 4: The results of applying tempGP and regGP on the simulated datasets with different strengths of autocorrelation

| $\phi$ | Average % improvement | Minimum % improvement | Maximum % improvement | Fraction of positive improvement |
|--------|-----------------------|-----------------------|-----------------------|----------------------------------|
| 0.5    | 0                     | -1.67                 | 6.08                  | 0.34                             |
| 1      | 3.04                  | -1.87                 | 28.42                 | 0.61                             |
| 1.5    | 10.23                 | -1.11                 | 40.58                 | 0.82                             |
| 2      | 14.29                 | -1.71                 | 58.45                 | 0.94                             |
| 2.5    | 14.91                 | -9.71                 | 48.56                 | 0.96                             |
| 3      | 13.34                 | -6.62                 | 45.52                 | 0.93                             |
| 3.5    | 12.45                 | -4.05                 | 42.72                 | 0.96                             |
| 4      | 12.47                 | -6.06                 | 44.34                 | 0.95                             |
| 4.5    | 9.11                  | -2.44                 | 41.06                 | 0.94                             |
| 5      | 8.63                  | -3.86                 | 29.45                 | 0.92                             |

(RMSE) of tempGP and regGP. We summarize the results of all the simulation runs in Table 4. The first column of the table is the lengthscale parameter  $\phi$ , which denotes the strength of the autocorrelation in the errors. The second, third and fourth columns are the average, minimum, and maximum percentage improvement for tempGP over regGP, respectively. The last column is the fraction of runs (out of 100) for which tempGP does better than regGP. We can see from the table that the average improvement increases as the strength of autocorrelation increases upto a certain value ( $\phi = 2.5$  in this case) and then starts decreasing. This is attributed to the fact that for a very small value of autocorrelation, the data is as good as independent. Thus, tempGP does not provide any significant improvement over regGP. As the strength of autocorrelation increases, the advantage of tempGP becomes more pronounced. After a certain value of  $\phi$ , the autocorrelation gradually moves from short-range dependence to long-range dependence (Opsomer et al., 2001), where the autocorrelation cannot be effectively removed even after thinning the dataset. Thus, tempGP’s performance gain starts to gradually go down. In other words, tempGP is more suited to handle the short-range dependence, which is the case for our intended application.

In order to view the distribution of the improvement, we also plot the histogram of percentage improvement the simulation runs with a few values of  $\phi$  in Figure 7.

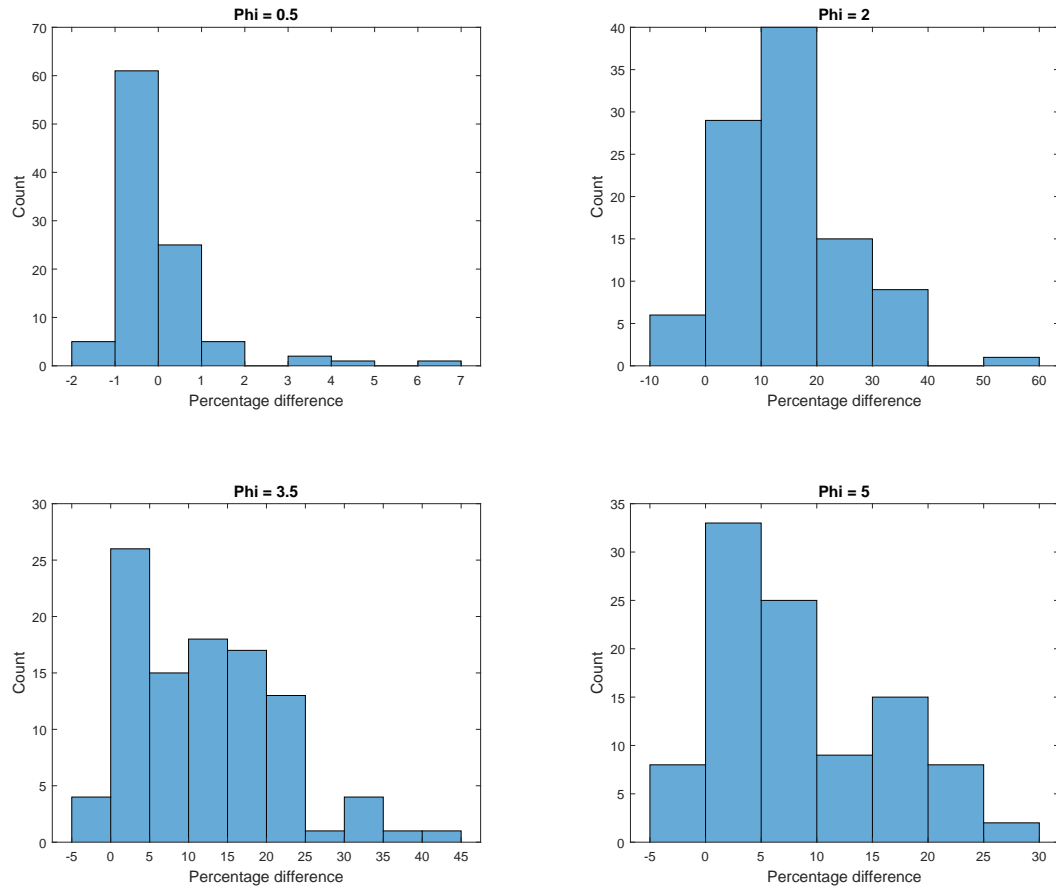

Figure 7: Histogram of percentage improvement for tempGP over regGP for different strengths of autocorrelation.

## References

Opsomer, J., Wang, Y., and Yang, Y. (2001). Nonparametric regression with correlated errors. *Statistical Science*, 16(2):134–153.
